# Supplementary material for: Hypergeometric SLE: Conformal Markov Characterization and Applications
Source: arXiv:1703.02022 source file (2018-02-24)
Supplement: Supplementary file 1 [file appendix_localsle.tex]

In this section, we summarize notation and properties of multiple local SLEs which were studied in \cite{DubedatCommutationSLE}. As we only need local $2$-$\SLE$, we restrict our notation to this particular case. We follow the framework described in \cite[Appendix]{KytolaPeltolaPurePartitionFunctions}. 

Fix a quad $q=(\Omega; x_1, x_2, x_3, x_4)$. The localization neighborhoods $U_1, \ldots, U_4$ are assumed to be closed subsets of $\overline{\Omega}$ such that $\Omega\setminus U_j$ are simply connected and $U_j\cap U_k=\emptyset$ for $j\neq k$. The local $2$-$\SLE_{\kappa}$ in $\Omega$, started from $(x_1, \ldots, x_4)$ and localized in $(U_1, \ldots, U_4)$ is a probability measure on $4$-tuples of curves $(\gamma_1, \ldots, \gamma_4)$ such that, for each $j$, the curve $\gamma_j$ starts at $x_j$ and ends when exiting $U_j$. The local $2$-$\SLE_{\kappa}$ is the indexed collection 
\[P=\left(P_{(q; U_1, \ldots, U_4)}\right)_{q; U_1, \ldots, U_4}.\]
This collection of probability measures is required to satisfy the following three properties.
